# Supplementary material for: A Hybrid Framework Using a QUBO Solver For Permutation-Based Combinatorial Optimization
Source: arXiv:2009.12767 source file (2021-07-06)
Supplement: Supplementary file 1 [file Supplement.tex]

\section{Supplement}

The first two moments for the perturbed distances are 

\begin{equation}M_1 = \frac{\sum_{i=1}\sum_{j \ne i} d_{ij} + \Delta_i + \Delta_j}{n^2-n}\end{equation}

and

\begin{equation}M_2 = \frac{\sum_{i=1}\sum_{j \ne i} (d_{ij} + \Delta_i + \Delta_j)^2}{n^2-n}.\end{equation}

Hence, the variance is 

\begin{align}V &= M_2 - M_1^2 \\&= \frac{\sum_{i=1}\sum_{j \ne i} (d_{ij} + \Delta_i + \Delta_j)^2}{n^2-n} \\&- \left[\frac{\sum_{i=1}\sum_{j \ne i} d_{ij} + \Delta_i + \Delta_j}{n^2-n}\right]^2.\end{align}

Consider a particular index $k$,

\begin{align}
&\frac{\partial V}{\partial \Delta_k} \\
&= \frac{2 \sum_{j \ne k}^n [d_{kj}+\Delta_k + \Delta_j + d_{jk} + \Delta_j + \Delta_k]}{n^2-n} \\&- \frac{2}{(n^2-n)^2}[\sum_{i=1}^n \sum_{j \ne i} d_{ij} + \Delta_i + \Delta_j] \frac{\partial}{\partial \Delta_k} \left[ \sum_{i=1}^n \sum_{j \ne i} d_{ij} + \Delta_i + \Delta_j \right]\\
&= \frac{2 \sum_{j \ne k}^n [d_{kj}+\Delta_k + \Delta_j + d_{jk} + \Delta_j + \Delta_k]}{n^2-n} \\&- \frac{4(n-1)}{(n^2-n)^2}[\sum_{i=1}^n \sum_{j \ne i} (d_{ij} + \Delta_i + \Delta_j)]  \\
&= \frac{2 \sum_{j \ne k}^n (d_{kj}+d_{jk}) + 4 \sum_{j \ne k}^n (\Delta_j + \Delta_k)}{n^2-n} \\&- \frac{4(n-1)}{(n^2-n)^2}[\sum_{i=1}^n \sum_{j \ne i} d_{ij} + \sum_{i=1}^n \sum_{j \ne i}(\Delta_i + \Delta_j)]  \\
&= \frac{2 \sum_{j \ne k}^n (d_{kj}+d_{jk}) + 4(n-1) \Delta_k +4 \sum_{j \ne k}^n \Delta_j}{n^2-n} \\&- \frac{4(n-1)}{n^2(n-1)^2}[\sum_{i=1}^n \sum_{j \ne i} d_{ij} + 2(n-1)\sum_{i=1}^n \Delta_i] 
\end{align}

We set the above expression to $0$ and simplify it.

\begin{align}&\sum_{j \ne k}^n (d_{kj}+d_{jk}) + 2(n-1) \Delta_k + 2 \sum_{j \ne k}^n \Delta_j \\&= \frac2n \left[ \sum_{i=1}^n\sum_{j \ne i} d_{ij}+ 2(n-1)\sum_{i=1}^n \Delta_i\right]\end{align}

%$$\sum_{j \ne k}^n (d_{kj}+d_{jk}) + 2(n-2) \Delta_k + 2 \sum_{j =1}^n \Delta_j = \frac2n  \sum_{i=1}^n\sum_{j \ne i} d_{ij}+ \frac{4(n-1)}{n}\sum_{i=1}^n \Delta_i$$

Collecting all the unknowns to one side, we get:
\begin{align}&2(n-2)\Delta_k + \left[ 2-\frac{4(n-1)}n\right]\sum_{j=1}^n \Delta_j \\&= \frac2n \left[ \sum_{i=1}^n \sum_{j \ne i} d_{ij}\right] - \sum_{j \ne k}^n (d_{kj}+d_{jk})\end{align}

Dividing by $2$ on both sides gives us
\begin{align}&\left(1-\frac1n \right)\Delta_k + \left[ -\frac{1}n\right]\sum_{j\ne k}^n \Delta_j \\&=\frac1{(n-2)} \left(\frac1n \left[ \sum_{i=1}^n \sum_{j \ne i} d_{ij}\right] - \frac12\sum_{j \ne k}^n (d_{kj}+d_{jk})\right) \end{align}

That is we can solve a linear system to obtain a solution. This is expected as we differentiated a quadratic function to get the optimal perturbation to minimize variance. Another reason why this is expected as changing all the distances by the same constant doesn't change the variance.

%The linear system is not invertible but we can solve for the least square solution for the matrix system.
%While the system is not invertible (again, this is expected as we can always add constant to every distances and preserve the variance), we can pick it to be the least square solution provided by most linear solvers. %A remark about this matrix is that this is a rate transition matrix.

%After which, we can set the minimum to $0$.

%This approach however might give us non-integer solutions.

%Another note is that if such trick were to apply to problem to problem such as Quadratic Assignment Problem directly (QAP), we will end up with a system of cubic equations where each such cubic equation can be factorize into a linear and a quadratic expression. Rather than directly solving the system, a possible estimation is that we can perform the least square approximation on the flow matrix and the distance matrix separately and the n join them together.

\textbf{Small Instance}

\begin{center}
\begin{tabular}{ |c|c| } 
\hline 
Parameter & Setting \\
\hline 
$A$ & 	$[\max(d_{ij}), 1.5 \cdot \max(d_{ij})]$, step $=5$\\ 
\hline
$B$&	1 \\ \hline
\end{tabular}
\end{center}

\textbf{Large Instance}

\begin{center}
\begin{tabular}{ |c|c| } 
\hline 
Parameter & Setting \\
\hline 
$A$ & 	$[2.5 \cdot \text{mean}(d_{ij}), 2 \cdot \max(d_{ij})]$, step $=150$\\ 
\hline
$B$&	2 \\ \hline
\end{tabular}
\end{center}

%The step size of $A$ is only applicable when we do not use HyperOpt to find the tuning parameter.

\subsection{Small Instance}

We test our approach on the problem size of number of jobs $ \in [10,20,30]$ and number of machines$ \in [5,10]$ and three different distance matrix formulation are tested. The results are shown below:

\subsubsection{$10$ Jobs $5$ Machines}
\begin{center}
\begin{tabular}{|c|c|c|c|c|c|} \hline
Test Case &	NEH	& \begin{tabular}{@{}c@{}} Residual  \\ Square\end{tabular} & \begin{tabular}{@{}c@{}}	Residual \\
No Carry \end{tabular} &	SPIRIT	& FSHOPH \\ \hline
VFR10\_5\_1\_Gap &	695	& \textbf{695}&	707	&710&	696 \\ \hline
VFR10\_5\_2\_Gap&	718	&\textbf{732}	&\textbf{732} &	744	&737\\ \hline
VFR10\_5\_3\_Gap&	754	&741	&\textbf{737}&	741&	742\\\hline
VFR10\_5\_4\_Gap&	703	&709	&\textbf{703}&	743&	709\\\hline
VFR10\_5\_5\_Gap&	770	&\textbf{738}	&\textbf{738}&	766&	\textbf{738}\\\hline
VFR10\_5\_6\_Gap&	748	&\textbf{770}	&779&	\textbf{770}&	\textbf{770}\\\hline
VFR10\_5\_7\_Gap&	754	&\textbf{744}	&760&	747&	755\\\hline
VFR10\_5\_8\_Gap&	705	&696	&704&	704&	\textbf{689}\\\hline
VFR10\_5\_9\_Gap&	787	&802	&783&	810&	\textbf{771}\\\hline
VFR10\_5\_10\_Gap&	664	&\textbf{669}	&677&	729&	685\\\hline
\end{tabular}
\end{center}

\begin{center}
\begin{tabular}{ |c|c|c|c|c| } 
\hline
\begin{tabular}{@{}c@{}} Distance  \\ Formulation\end{tabular}
 & \begin{tabular}{@{}c@{}} Residual \\ Square\end{tabular}
 &  	 \begin{tabular}{@{}c@{}} Residual \\ No Carry    \end{tabular}& SPIRIT & FSHOPH \\
\hline
avg \% & 	$-0.01\%$ &	$-0.25\%$  & $2.38\% $&  $\textbf{-0.37\%}$ \\ 
\hline
\end{tabular}
\end{center}

\subsubsection{$10$ Jobs $10$ Machines}

\begin{center}
\begin{tabular}{|c|c|c|c|c|c|} \hline
Test Case &	NEH	& \begin{tabular}{@{}c@{}} Residual  \\ Square\end{tabular} & \begin{tabular}{@{}c@{}}	Residual \\
No Carry \end{tabular} &	SPIRIT	& FSHOPH \\ \hline
VFR10\_10\_1\_Gap &	1160&	\textbf{1128}&	1176&	1188&	1158 \\ \hline
VFR10\_10\_2\_Gap&	1157&	\textbf{1166}&	1173&	\textbf{1166}&	1177\\ \hline
VFR10\_10\_3\_Gap&	1149&	\textbf{1143}&	1146&	1173&	1155\\\hline
VFR10\_10\_4\_Gap&	1049&	1120&	\textbf{1109}&	1115&	1103\\\hline
VFR10\_10\_5\_Gap&	1126&	\textbf{1113}&	1126&	1141&	1139\\\hline
VFR10\_10\_6\_Gap&	1104&	1099&	1100&	\textbf{1098}&	1129\\\hline
VFR10\_10\_7\_Gap&	1117&	1164&	\textbf{1162}&	1179&	1181\\\hline
VFR10\_10\_8\_Gap&	1129&	1150&	\textbf{1131}&	1158&	1151\\\hline
VFR10\_10\_9\_Gap&	1052&	\textbf{1076}&	1091&	1117&	1091\\\hline
VFR10\_10\_10\_Gap&	1118&	1158&	1146&	\textbf{1116}&	1147\\\hline
\end{tabular}
\end{center}

\begin{center}
\begin{tabular}{ |c|c|c|c|c| } 
\hline
\begin{tabular}{@{}c@{}} Distance  \\ Formulation\end{tabular}
 & \begin{tabular}{@{}c@{}} Residual \\ Square\end{tabular}
 &  	 \begin{tabular}{@{}c@{}} Residual \\ No Carry    \end{tabular}& SPIRIT & FSHOPH \\
\hline
avg \% & 	$\textbf{1.46\%}$ &	$1.83\%$  & $2.65\% $&  $2.46\%$ \\ 
\hline
\end{tabular}
\end{center}

\subsubsection{$20$ Jobs $5$ Machines}

\begin{center}
\begin{tabular}{|c|c|c|c|c|c|} \hline
Test Case &	NEH	& \begin{tabular}{@{}c@{}} Residual  \\ Square\end{tabular} & \begin{tabular}{@{}c@{}}	Residual \\
No Carry \end{tabular} &	SPIRIT	& FSHOPH \\ \hline
VFR20\_5\_1\_Gap &	1214&	1253&	1256&	1267&	\textbf{1251} \\ \hline
VFR20\_5\_2\_Gap&	1290&	\textbf{1325}&	1302&	1316&	1357\\ \hline
VFR20\_5\_3\_Gap&	1352&	1406&	\textbf{1399}&	1419&	1455\\\hline
VFR20\_5\_4\_Gap&	1178&	\textbf{1187}&	1226&	1217&	1220\\\hline
VFR20\_5\_5\_Gap&	1375&	1380&	1398&	\textbf{1378}&	1418\\\hline
VFR20\_5\_6\_Gap&	1095&	1167&	\textbf{1137}&	1145&	1180\\\hline
VFR20\_5\_7\_Gap&	1163&	1212&	1216&	\textbf{1207}&	1238\\\hline
VFR20\_5\_8\_Gap&	1127&	\textbf{1160}&	1206&	1161&	1207\\\hline
VFR20\_5\_9\_Gap&	1321&	1361&	1369&	\textbf{1343}&	1370\\\hline
VFR20\_5\_10\_Gap&	1289&	\textbf{1322}&	1341&	1342&	1348\\\hline
\end{tabular}
\end{center}

\begin{center}
\begin{tabular}{ |c|c|c|c|c| } 
\hline
\begin{tabular}{@{}c@{}} Distance  \\ Formulation\end{tabular}
 & \begin{tabular}{@{}c@{}} Residual \\ Square\end{tabular}
 &  	 \begin{tabular}{@{}c@{}} Residual \\ No Carry    \end{tabular}& SPIRIT & FSHOPH \\
\hline
avg \% & 	$\textbf{3.03\%}$ &	$3.67\%$  & $3.21\% $&  $5.21\%$ \\ 
\hline
\end{tabular}
\end{center}

\subsubsection{$20$ Jobs $10$ Machines}
\begin{center}
\begin{tabular}{|c|c|c|c|c|c|} \hline
Test Case &	NEH	& \begin{tabular}{@{}c@{}} Residual  \\ Square\end{tabular} & \begin{tabular}{@{}c@{}}	Residual \\
No Carry \end{tabular} &	SPIRIT	& FSHOPH \\ \hline
VFR20\_10\_1\_Gap &	1690&	\textbf{1705}&	1707&	1710&	1749 \\ \hline
VFR20\_10\_2\_Gap&	1600&	1687&	\textbf{1671}&	1680&	1699\\ \hline
VFR20\_10\_3\_Gap&	1667&	1781&	1790&	\textbf{1768}&	1798\\\hline
VFR20\_10\_4\_Gap&	1481&	1623&	\textbf{1553}&	1677&	1606\\\hline
VFR20\_10\_5\_Gap&	1663&	1758&	\textbf{1751}&	1783&	1787\\\hline
VFR20\_10\_6\_Gap&	1682&	1810&	1789&	\textbf{1747}&	1810\\\hline
VFR20\_10\_7\_Gap&	1679&	\textbf{1717}&	1728&	1784&	1789\\\hline
VFR20\_10\_8\_Gap&	1608&	\textbf{1718}&	1736&	1744&	1723\\\hline
VFR20\_10\_9\_Gap&	1620&	1664&	\textbf{1627}&	1669&	1740\\\hline
VFR20\_10\_10\_Gap&	1569&	1692&	1682&	\textbf{1675}&	\textbf{1675}\\\hline
\end{tabular}
\end{center}

\begin{center}
\begin{tabular}{ |c|c|c|c|c| } 
\hline
\begin{tabular}{@{}c@{}} Distance  \\ Formulation\end{tabular}
 & \begin{tabular}{@{}c@{}} Residual \\ Square\end{tabular}
 &  	 \begin{tabular}{@{}c@{}} Residual \\ No Carry    \end{tabular}& SPIRIT & FSHOPH \\
\hline
avg \% & 	$5.57\%$ &	$\textbf{4.79\%}$  & $6.12\% $&  $6.89\%$ \\ 
\hline
\end{tabular}
\end{center}

\subsubsection{$30$ Jobs $5$ Machines}
\begin{center}
\begin{tabular}{|c|c|c|c|c|c|} \hline
Test Case &	NEH	& \begin{tabular}{@{}c@{}} Residual  \\ Square\end{tabular} & \begin{tabular}{@{}c@{}}	Residual \\
No Carry \end{tabular} &	SPIRIT	& FSHOPH \\ \hline
VFR30\_5\_1\_Gap &	1820&	1884&	\textbf{1840}&	1863&	1912 \\ \hline
VFR30\_5\_2\_Gap&	1608&	1683&	\textbf{1665}&	1703&	1684\\ \hline
VFR30\_5\_3\_Gap&	1730&	1802&	\textbf{1767}&	1812&	1840\\\hline
VFR30\_5\_4\_Gap&	1791&	1864&	1858&	1879&	\textbf{1847}\\\hline
VFR30\_5\_5\_Gap&	1743&	1786&	\textbf{1766}&	1795&	1850\\\hline
VFR30\_5\_6\_Gap&	1878&	1909&	\textbf{1877}&	1927&	1911\\\hline
VFR30\_5\_7\_Gap&	1749&	1807&	\textbf{1782}&	1797&	1812\\\hline
VFR30\_5\_8\_Gap&	1736&	\textbf{1795}&	1840&	1830&	1860\\\hline
VFR30\_5\_9\_Gap&	1735&	1819&	\textbf{1781}&	1826&	1794\\\hline
VFR30\_5\_10\_Gap&	1666&	1739&	1745&	\textbf{1721}&	1770\\\hline
\end{tabular}
\end{center}

\begin{center}
\begin{tabular}{ |c|c|c|c|c| } 
\hline
\begin{tabular}{@{}c@{}} Distance  \\ Formulation\end{tabular}
 & \begin{tabular}{@{}c@{}} Residual \\ Square\end{tabular}
 &  	 \begin{tabular}{@{}c@{}} Residual \\ No Carry    \end{tabular}& SPIRIT & FSHOPH \\
\hline
avg \% & 	$3.65\%$ &	$\textbf{2.71\%}$  & $4.02\% $&  $4.76\%$ \\ 
\hline
\end{tabular}
\end{center}

\subsubsection{$30$ Jobs $10$ Machines}

\begin{center}
\begin{tabular}{|c|c|c|c|c|c|} \hline
Test Case &	NEH	& \begin{tabular}{@{}c@{}} Residual  \\ Square\end{tabular} & \begin{tabular}{@{}c@{}}	Residual \\
No Carry \end{tabular} &	SPIRIT	& FSHOPH \\ \hline
VFR30\_10\_1\_Gap &	2039&	2239&	2220&	\textbf{2196}&	2274 \\ \hline
VFR30\_10\_2\_Gap&	2182&	2410&	2385&	\textbf{2370}&	2426\\ \hline
VFR30\_10\_3\_Gap&	2222&	\textbf{2335}&	2368&	2366&	2389\\\hline
VFR30\_10\_4\_Gap&	2077&	2272&	\textbf{2216}&	2240&	2275\\\hline
VFR30\_10\_5\_Gap&	2134&	2233&	\textbf{2314}&	2346&	2328\\\hline
VFR30\_10\_6\_Gap&	2126&	\textbf{2325}&	2334&	2377&	2356\\\hline
VFR30\_10\_7\_Gap&	2075&	2218&	2258&	\textbf{2203}&	2275\\\hline
VFR30\_10\_8\_Gap&	2008&	2126&	\textbf{2120}&	2152&	2190\\\hline
VFR30\_10\_9\_Gap&	1962&	\textbf{2162}&	2186&	2221&	2246\\\hline
VFR30\_10\_10\_Gap&	2043&	\textbf{2111}&	2197&	2180&	2233\\\hline
\end{tabular}
\end{center}

\begin{center}
\begin{tabular}{ |c|c|c|c|c| } 
\hline
\begin{tabular}{@{}c@{}} Distance  \\ Formulation\end{tabular}
 & \begin{tabular}{@{}c@{}} Residual \\ Square\end{tabular}
 &  	 \begin{tabular}{@{}c@{}} Residual \\ No Carry    \end{tabular}& SPIRIT & FSHOPH \\
\hline
avg \% & 	$\textbf{7.5\%}$ &	$8.30\%$  & $8.56\% $&  $10.22\%$ \\ 
\hline
\end{tabular}
\end{center}

From the experiment results on small scale problems, we could see that the two distance formulations which are Residual Square and Residual No carry have better performance compared with others. The average percentage off the NEH solution are all below $10\%$. Note that the previous results are only tested once on each test instances.

\subsection{Large Instance}

We test our approach on the problem size of number of jobs=200 and number of machines$\in [20,40,60]$ and three different distance matrix formulation are tested. The results are shown below:

\subsubsection{$200$ Jobs $20$ Machines}
\begin{center}
\begin{tabular}{|c|c|c|c|c|c|} \hline
Test Case &	NEH	& \begin{tabular}{@{}c@{}} Residual  \\ Square\end{tabular} & \begin{tabular}{@{}c@{}}	Residual \\
No Carry \end{tabular} &	SPIRIT	& FSHOPH \\ \hline
VFR200\_20\_1\_Gap &	11931&	13152&	\textbf{12978}&	13278&	13152\\ \hline
VFR200\_20\_2\_Gap&	11834&	\textbf{12891}&	12948&	13216&	12971\\ \hline
VFR200\_20\_3\_Gap&	11826&	13157&	13129&	13188&	\textbf{13080}\\\hline
VFR200\_20\_4\_Gap&	11662&	13095&	12927&	13116&	\textbf{12870}\\\hline
VFR200\_20\_5\_Gap&	11643&	13129&	12989&	13057&	\textbf{12863}\\\hline
VFR200\_20\_6\_Gap&	11798&	13053&	13212&	13024&	\textbf{12966}\\\hline
VFR200\_20\_7\_Gap&	11759&	13241&	\textbf{12935}&	13304&	13140\\\hline
VFR200\_20\_8\_Gap&	11539&	12686&	12730&	13355&	\textbf{12683}\\\hline
VFR200\_20\_9\_Gap&	11608&	12799&	12797&	\textbf{12589}&	12895\\\hline
VFR200\_20\_10\_Gap&	11798&	13006&	13002&	13063&	\textbf{12876}\\\hline
\end{tabular}
\end{center}

\begin{center}
\begin{tabular}{ |c|c|c|c|c| } 
\hline
\begin{tabular}{@{}c@{}} Distance  \\ Formulation\end{tabular}
 & \begin{tabular}{@{}c@{}} Residual \\ Square\end{tabular}
 &  	 \begin{tabular}{@{}c@{}} Residual \\ No Carry    \end{tabular}& SPIRIT & FSHOPH \\
\hline
avg \% & 	$10.92\%$ &	$10.44\%$  & $11.75\% $&  $\textbf{10.31\%}$ \\ 
\hline
\end{tabular}
\end{center}

\subsubsection{$200$ Jobs $40$ Machines}
\begin{center}
\begin{tabular}{|c|c|c|c|c|c|} \hline
Test Case &	NEH	& \begin{tabular}{@{}c@{}} Residual  \\ Square\end{tabular} & \begin{tabular}{@{}c@{}}	Residual \\
No Carry \end{tabular} &	SPIRIT	& FSHOPH \\ \hline
VFR200\_40\_1\_Gap &	13769&	15349&	15047&	15229&	\textbf{14973}\\ \hline
VFR200\_40\_2\_Gap&	13687&	15144&	15060&	\textbf{15055}&	15072\\ \hline
VFR200\_40\_3\_Gap&	13853&	15338&	\textbf{15044}&	15355&	15147\\\hline
VFR200\_40\_4\_Gap&	13877&	15166&	\textbf{14991}&	15277&	15061\\\hline
VFR200\_40\_5\_Gap&	13610&	15080&	\textbf{15050}&	15200&	15156\\\hline
VFR200\_40\_6\_Gap&	13695&	15210&	\textbf{15059}&	15420&	15103\\\hline
VFR200\_40\_7\_Gap&	13874&	15466&	15351&	15332&	\textbf{15204}\\\hline
VFR200\_40\_8\_Gap&	13850&	15200&	15211&	15265&	\textbf{15080}\\\hline
VFR200\_40\_9\_Gap&	13724&	15143&	15118&	15190&	\textbf{15032}\\\hline
VFR200\_40\_10\_Gap& 13858&	15403&	15278&	15232&	\textbf{15176}\\\hline
\end{tabular}
\end{center}

\begin{center}
\begin{tabular}{ |c|c|c|c|c| } 
\hline
\begin{tabular}{@{}c@{}} Distance  \\ Formulation\end{tabular}
 & \begin{tabular}{@{}c@{}} Residual \\ Square\end{tabular}
 &  	 \begin{tabular}{@{}c@{}} Residual \\ No Carry    \end{tabular}& SPIRIT & FSHOPH \\
\hline
avg \% & 	$10.67\%$ &	$9.73\%$  & $10.71\% $&  $\textbf{9.59\%}$ \\ 
\hline
\end{tabular}
\end{center}

\subsubsection{$200$ Jobs $60$ Machines}
\begin{center}
\begin{tabular}{|c|c|c|c|c|c|} \hline
Test Case &	NEH	& \begin{tabular}{@{}c@{}} Residual  \\ Square\end{tabular} & \begin{tabular}{@{}c@{}}	Residual \\
No Carry \end{tabular} &	SPIRIT	& FSHOPH \\ \hline
VFR200\_60\_1\_Gap &	15716&	17215&	17094&	17306&	\textbf{17090}\\ \hline
VFR200\_60\_2\_Gap&	15636&	17223&	17192&	17123&	\textbf{16968}\\ \hline
VFR200\_60\_3\_Gap&	15969&	17256&	17296&	17181&	17092\\\hline
VFR200\_60\_4\_Gap&	15734&	17321&	17275&	17279&	\textbf{17156}\\\hline
VFR200\_60\_5\_Gap&	15801&	17255&	17217&	17519&	\textbf{17100}\\\hline
VFR200\_60\_6\_Gap&	15733&	17193&	17110&	17157&	\textbf{17064}\\\hline
VFR200\_60\_7\_Gap&	15743&	17244&	17329&	17186&	\textbf{17121}\\\hline
VFR200\_60\_8\_Gap&	15633&	17263&	\textbf{17060}&	17289&	17181\\\hline
VFR200\_60\_9\_Gap&	15606&	16967&	17084&	17074&	\textbf{16929}\\\hline
VFR200\_60\_10\_Gap& 15645&	16965&	17130&	17347&	\textbf{16952}\\\hline
\end{tabular}
\end{center}

\begin{center}
\begin{tabular}{ |c|c|c|c|c| } 
\hline
\begin{tabular}{@{}c@{}} Distance  \\ Formulation\end{tabular}
 & \begin{tabular}{@{}c@{}} Residual \\ Square\end{tabular}
 &  	 \begin{tabular}{@{}c@{}} Residual \\ No Carry    \end{tabular}& SPIRIT & FSHOPH \\
\hline
avg \% & 	$9.34\%$ &	$9.29\%$  & $9.70\% $&  $\textbf{8.55\%}$ \\ 
\hline
\end{tabular}
\end{center}

For large scale FSP, we observe that FSHOP has better performance compared with other $3$ distance formulations and the average percentage off NEH solution are below $10\%$.% However, the decomposition results are not unique. %Therefore, the performance may be improved by increasing the number of runs. 

%\subsection{Results and Conclusions for application of DA on FSP}

%From experiment results, we could see DA can solve the FSP by using analogy of TSP and it can derive good solution in terms of the quality and the solution time. Three different formulations of the distance matrix can be chosen to be applied based on the size of the problem. Besides, the limitation of the number of binary bits DA has is overcome by conducting decomposition technique i.e., spectral clustering which transform the original FSP into solving several smaller independent FSP. And the reconstruction of the original solution proves that the decomposition technique proposed does not harm the optimality of the original problem. 
%Other contributions including the implementation of the Python classes of Job, Sequence which could be used in the future research. The efficiency of the makespan calculation has been optimized using Python library Numba.

%One possible improvement we could make in the future is that we could compare the DA solution with some improved NEH algorithm even with some exact solver such as CPLEX and Gurobi. By comparing the DA solution with a better upper bound and the exact optimal solution may provide us more insights of the approach proposed in this project. 
%Besides, we could try to solve other types of the FSP including no-wait, limited buffer by applying similar strategy of transform them into TSP.
% Finally, we could investigate deeper about the decomposition method except the spectral clustering to get more robust and stable clustering results.
