# Supplementary material for: A Hybrid Framework Using a QUBO Solver For Permutation-Based Combinatorial Optimization
Source: arXiv:2009.12767 source file (2021-07-06)
Supplement: Supplementary file 2 [file supplementary.tex]

\newpage
 
 \textbf{Supplementary Document}
 
 \section{Data Scaling for General Sum to Constant Constraint}

In this appendix, we go beyond the setting of permutation constraints and discuss the data scaling for general permutation constraints.

Consider the following quadratic programming problem with binary variables.

\begin{equation}\label{originalobj}\min \sum_{\substack{u, v \in I\\ i, j \in J}} x_{u,i}Q_{u, i, v, j}x_{v,j}  \end{equation}

\noindent subject to 
$\sum_{u \in I} x_{u,i}=B$ and
$\sum_{i \in J} x_{u,i}=C$
where $|J|B = |I|C$.
That is we impose the conditions that the row sum is a constant and the column sum is another constant and the problem is feasible.

Let $\hat{j} \in J$.
Consider the optimization problem with scaled data:

\begin{equation}\label{perturbobj}\min \sum_{\substack{u,v \in I\\ i, j \in J}} x_{u,i}\tilde{Q}_{u,i,v,j}x_{v, j} \end{equation}

subject to 
$\sum_{u \in I} x_{u,i}=B$ and
$\sum_{j \in J} x_{u,i}=C$ where

$$\forall u, v \in I, \forall J \in I \tilde{Q}_{i,j,u,v} = \begin{cases} Q_{u,i, v, j} & \text{if } j \ne \hat{j} \\ Q_{u,i, v, j} + \Delta & {if } j= \hat{j}\end{cases}$$

The following lemma shows that the ranking of optimality is preserved under data perturbation: 

\begin{lemma}
A solution $y$ that is better than $z$ for optimization problem $(\ref{originalobj})$ remains better for optimization problem $(\ref{perturbobj})$.
\end{lemma}
  
\begin{proof}
It suffices to show that the difference in the objective values of the two solutions $y$ and $z$ remain the same before and after data scaling. More precisely, 
\begin{align*}&\sum_{\substack{u, v \in I\\ i, j \in J}} z_{u, i}Q_{u, i,v, j}z_{v, j} -  \sum_{\substack{u, v \in I\\ i, j \in J}} y_{u, i}Q_{u, i, v, j}y_{v, j}\\&=\sum_{\substack{u, v \in I\\ i, j \in J}} z_{u, i}\tilde{Q}_{u, i, v, j}z_{v, j} -  \sum_{\substack{u, v \in I\\ i, j \in J}} y_{u, i}\tilde{Q}_{u, i, v, j}y_{v, j}.\end{align*}
 
By definition of $\tilde{Q}$, we have,
\begin{align*}
&\sum_{\substack{u, v \in I\\ i, j \in J} } z_{u, i}\tilde{Q}_{u, i, v, j} z_{v, j} - y_{u, i} \tilde{Q}_{u, i, j, v} y_{v, j} \\
&= \sum_{\substack{u, v \in I \\ i, j \in J}} [z_{u, i}Q_{u, i, v, j} z_{v, j} - y_{u, i}Q_{u, i, v, j} y_{v,j}] \\ \end{align*}
\begin{align}
&+\Delta \sum_{\substack{u, v \in I} ,i \in J} [z_{u,i} z_{v, \hat{j}} - y_{u, i} y_{v, \hat{j}}] \label{secondterm}
\end{align}

Since both solutions are feasible, i.e. 
$\sum_{u \in I} y_{u, i}=\sum_{i \in I} z_{u, i}=B$ and 
$\sum_{i \in J} y_{u, i}=\sum_{i \in J} z_{u, i}=C$,   we have

$$
\sum_{\substack{u, v \in I \\ i \in J}} y_{u, i}y_{v, \hat{j}} = \sum_{v \in I} y_{v ,\hat{j}} \sum_{u \in I} \sum_{i \in J} y_{i, u} = B \sum_{u \in I} C = BC|I|
$$
and similarly
$
\sum_{\substack{u, v \in I \\ i \in J}} z_{u, i}z_{v, \hat{j}}
= BC|I|
$

Hence the term $(\ref{secondterm})$ is equal to 0. 

%\begin{align*}
%&\sum_{\substack{i,u  \in I\\ j, v\in J}} y_{i,j}\tilde{Q}_{i,j,u,v} y_{u,v} - z_{i,j} \tilde{Q}_{i,j,u,v} z_{uv} \\
%&=\sum_{\substack{i,u  \in I\\ j, v\in J}} y_{i,j}Q_{i,j,u,v} y_{u,v} - z_{i,j} Q_{i,j,u,v} z_{uv} 
%\end{align*}

\end{proof}

Specifically when $B=C=1$, and the index set $I=J=\{ 1, \ldots, n\}$, we have the special case for permutation based optimization problems.

\section{Zooming Algorithm}

To gather sufficient training data for the MLP, we design a heuristic called the Zooming Algorithm, given as follows:
\begin{enumerate}
    \item Partition the parameter space into bins.
    \item Sample parameter from those bins and evaluate the bin's performance
    \item Zoom in the bin that gives the best performance and repeat the iterations.
\end{enumerate}

Each time we zoom into the bin, we increase the number of iterations. This is similar to the idea of multi-arm bandit problem where we explore the possible parameter space and then exploit the space upon finding a potentially better region that gives us better performance. The collected data are then used as the training data to build a neural network model.

Note that once the machine learning model has been built, we no longer require to try multiple parameter values; rather the trained model would output one parameter value for the QUBO model. Hence, this would reduce the computational cost significantly.
